# Supplementary material for: VERINA: Benchmarking Verifiable Code Generation
Source: arXiv:2505.23135 source file (2026-03-16)
Supplement: Supplementary file 1 [file postcond_plausible.tex]

\begin{figure}[H]
\begin{lstlisting}[
    language=lean,
    basicstyle=\ttfamily\tiny
]
-- !benchmark @start import type=llm_solution
import Std.Data.HashMap
open Std
-- !benchmark @end import
-- !benchmark @start postcond_aux
@[reducible, simp]
def count (xs : List Int) (y : Int) : Nat :=
    xs.foldl (fun acc x => if x = y then acc + 1 else acc) 0
-- !benchmark @end postcond_aux
@[reducible, simp]
def mostFrequent_postcond (xs : List Int) (result: Int) (h_precond : mostFrequent_precond (xs)) : Prop :=
  -- !benchmark @start postcond
  let cr := count xs result;
  0 < cr ∧
  ∀ y,
    let cy := count xs y;
    cy ≤ cr ∧
    (cy = cr → ∃ i j,
        i < xs.length ∧
        j < xs.length ∧
        xs.get? i = some result ∧
        xs.get? j = some y ∧
        i ≤ j
    )
  -- !benchmark @end postcond
\end{lstlisting}
    \caption{Example (\texttt{verina\_advanced\_55}): LLM-generated post-condition can not be directly evaluated with test case values but is testable by plausible}
    \label{app-ex:postcond_plausible}
\end{figure}

\smallsec{Plausible testing for complex specifications}
\Cref{app-ex:postcond_plausible} illustrates how our evaluation framework handles complex LLM-generated specifications that cannot be evaluated through direct evaluation of test cases.
The LLM-generated post-condition for finding the most frequent element contains nested quantifiers that make it non-decidable for direct evaluation against test cases.
However, after plugging in concrete test case values to the post-condition, the resulting instantiated formula can be evaluated using Lean's plausible tactic.
This allows our framework to assess whether the specification holds for specific inputs by systematically exploring the instantiated logical structure.
The plausible testing approach enables evaluation of specifications involving complex logical relationships that would otherwise be impossible to check automatically, demonstrating the effectiveness of our testing-based evaluation methodology for handling the wide spectrum of formal specifications generated by LLMs.
