# Supplementary material for: VERINA: Benchmarking Verifiable Code Generation
Source: arXiv:2505.23135 source file (2026-03-16)
Supplement: Supplementary file 3 [file reject_input_json.tex]

\begin{figure}
\begin{lstlisting}[
    language=json,
    basicstyle=\ttfamily\tiny
]
[
    {
        "input": {
            "s": "#[1]",
            "k": 2
        }
    }
]
\end{lstlisting}
    \caption{Caption}
    \label{fig:enter-label}
\end{figure}
