# Supplementary material for: VERINA: Benchmarking Verifiable Code Generation
Source: arXiv:2505.23135 source file (2026-03-16)
Supplement: Supplementary file 4 [file task_json.tex]

\begin{figure}
\begin{lstlisting}[
    language=json,
    basicstyle=\ttfamily\tiny
]
{
    "id": "verina_basic_29",
    "signature": {
        "name": "removeElement",
        "parameters": [
            {
                "param_name": "s",
                "param_type": "Array Int"
            },
            {
                "param_name": "k",
                "param_type": "Nat"
            }
        ],
        "return_type": "Array Int"
    },
    "description_file": "./description.txt",
    "lean_file": "./task.lean",
    "metadata": {
        "upstream": {
            "name": "dafny-synthesis",
            "link": "https://github.com/Mondego/dafny-synthesis",
            "task_id": "task_id_610"
        }
    },
    "test_file": "./test.json",
    "reject_inputs_file": "./reject_inputs.json"
}
\end{lstlisting}
    \caption{Caption}
    \label{fig:enter-label}
\end{figure}
