# Supplementary material for: VERINA: Benchmarking Verifiable Code Generation
Source: arXiv:2505.23135 source file (2026-03-16)
Supplement: Supplementary file 5 [file test_json.tex]

\begin{figure}
\begin{lstlisting}[
    language=json,
    basicstyle=\ttfamily\tiny
]
[
    {
        "input": {
            "s": "#[1, 2, 3, 4, 5]",
            "k": 2
        },
        "expected": "#[1, 2, 4, 5]",
        "unexpected": [
            "#[1, 2, 3, 5]",
            "#[1, 3, 4, 5]",
            "#[2, 3, 4, 5]"
        ]
    },
    {
        "input": {
            "s": "#[10, 20, 30, 40]",
            "k": 0
        },
        "expected": "#[20, 30, 40]",
        "unexpected": [
            "#[10, 30, 40]",
            "#[10, 20, 30, 40]",
            "#[20, 30, 40, 0]"
        ]
    },
    {
        "input": {
            "s": "#[10, 20, 30, 40]",
            "k": 3
        },
        "expected": "#[10, 20, 30]",
        "unexpected": [
            "#[20, 30, 40]",
            "#[10, 20, 40]",
            "#[10, 30, 40]"
        ]
    },
    {
        "input": {
            "s": "#[7]",
            "k": 0
        },
        "expected": "#[]",
        "unexpected": [
            "#[7]",
            "#[0]"
        ]
    }
]
\end{lstlisting}
    \caption{Caption}
    \label{fig:enter-label}
\end{figure}
